# Supplementary material for: Improved microgrid resiliency through distributionally robust optimization under a policy-mode framework
Source: arXiv:2210.12586 source file (2024-03-11)
Supplement: Supplementary file 1 [file Appendices.tex]

\appendix

\section{appendix section 1}

\subsection{subsection title}

\paragraph{paragraph title}

\section{appendix section 2}
